# Supplementary material for: Radiation reaction in strong fields from an alternative perspective
Source: arXiv:1408.4411 source file (2014-08-19)

**AN EXPERT IS A PERSON WHO HAS MADE ALL THE MISTAKES  
THAT CAN BE MADE IN A VERY NARROW FIELD.**

**NEILS BOHR**

HOW WONDERFUL THAT WE HAVE MET WITH A PARADOX.

NOW WE HAVE SOME HOPE OF MAKING PROGRESS.

NEILS BOHR

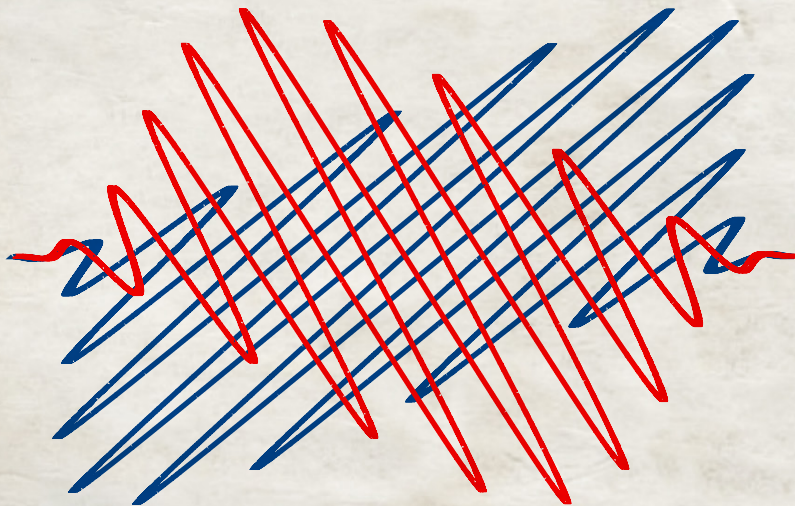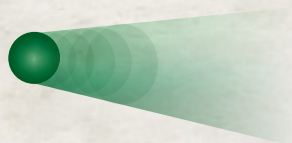

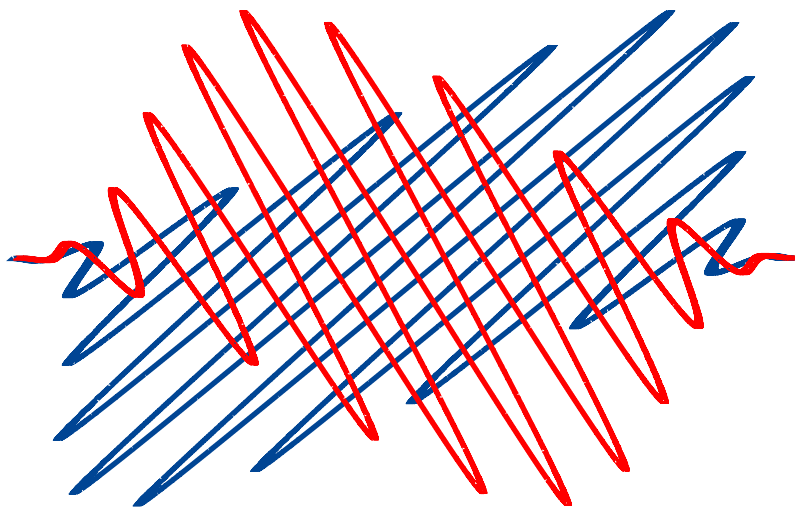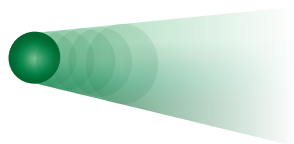

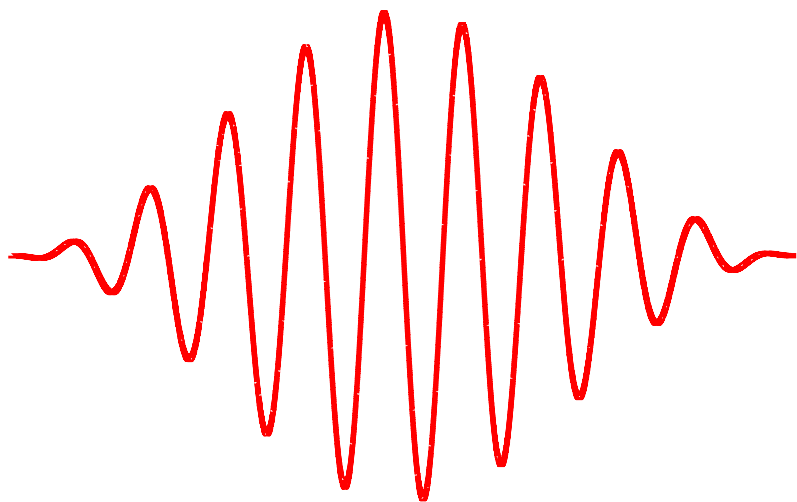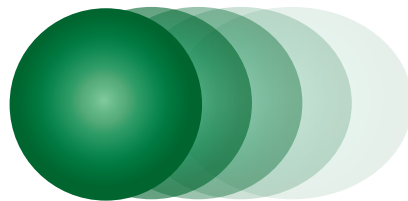

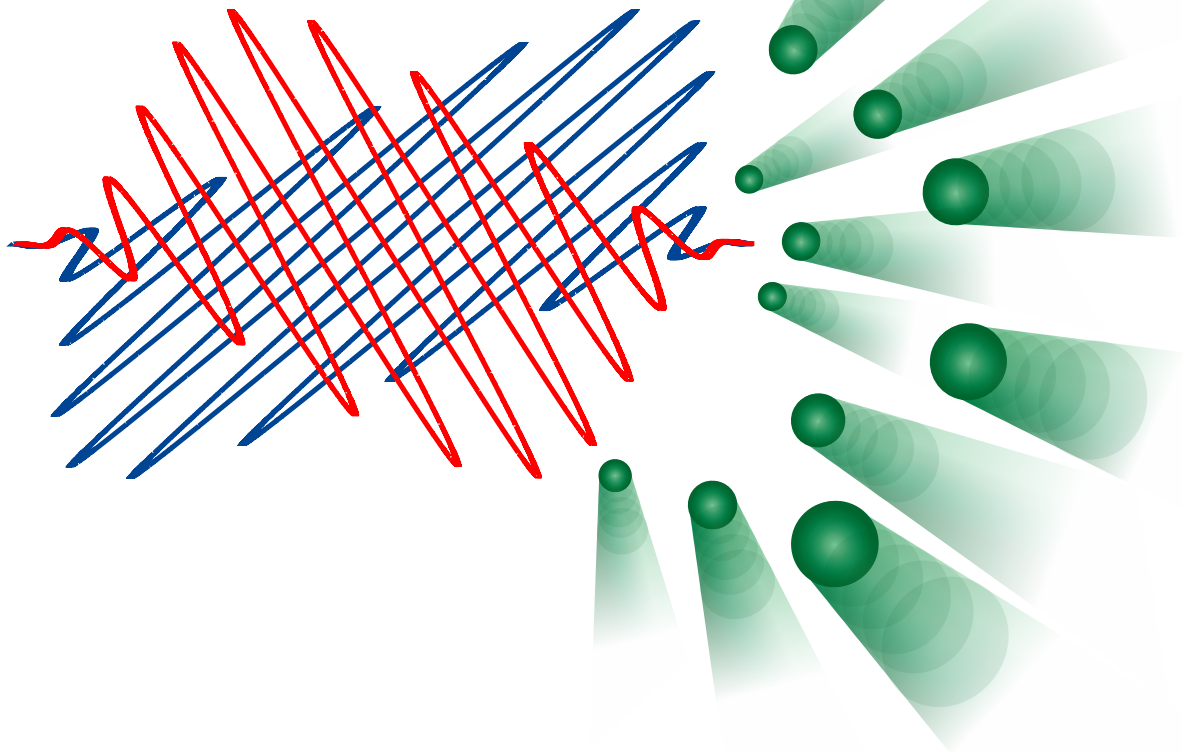



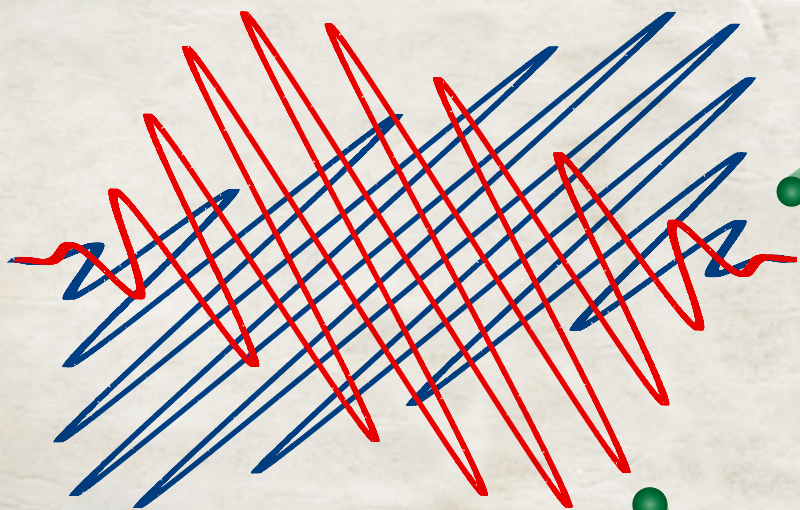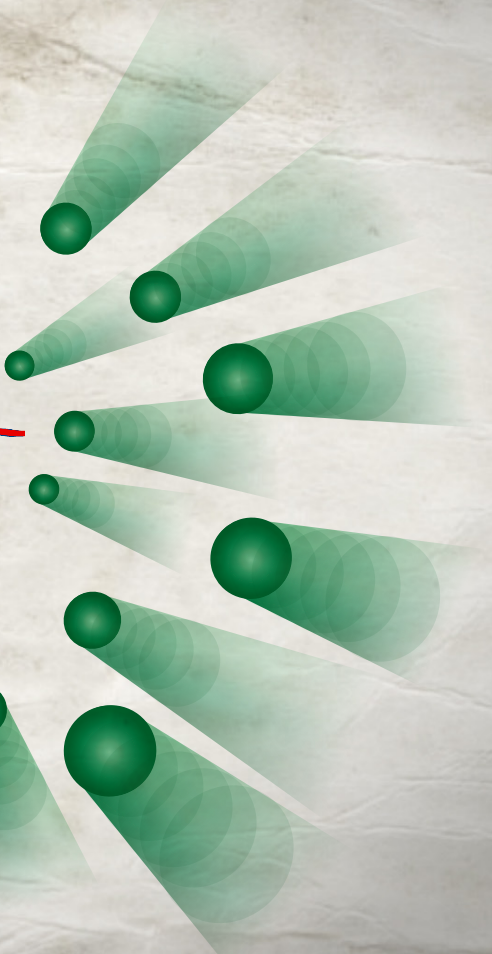

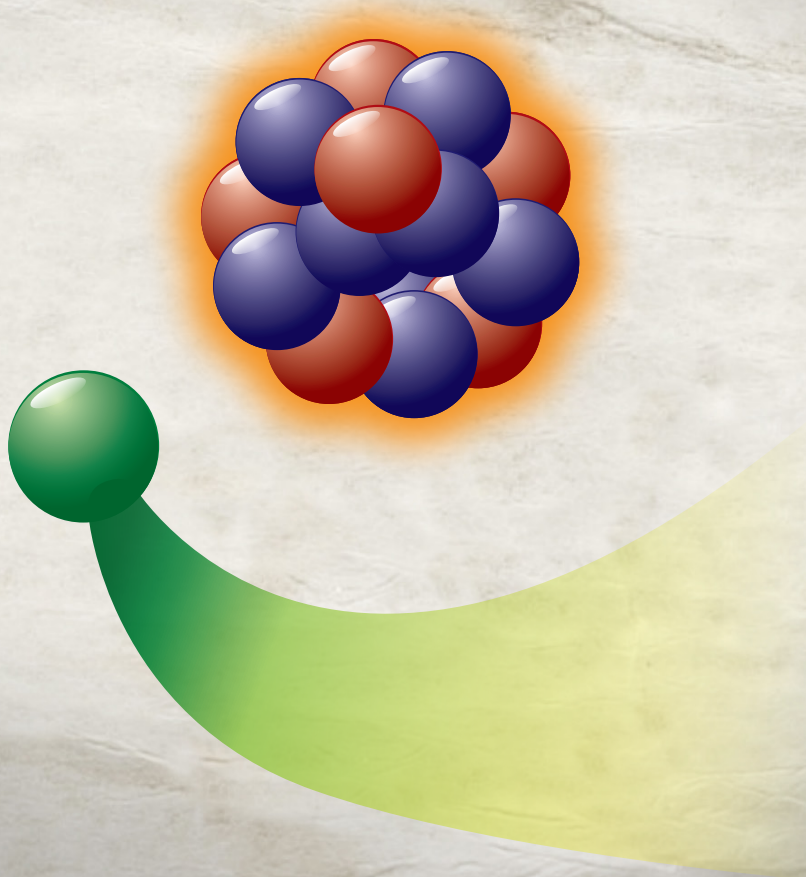



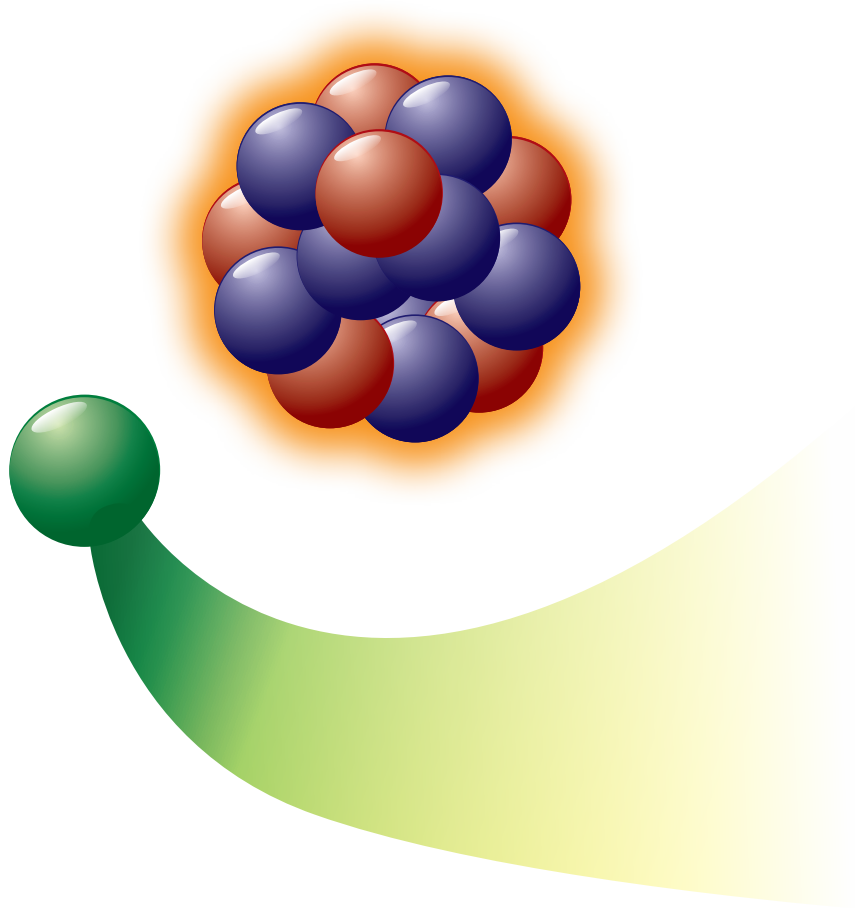

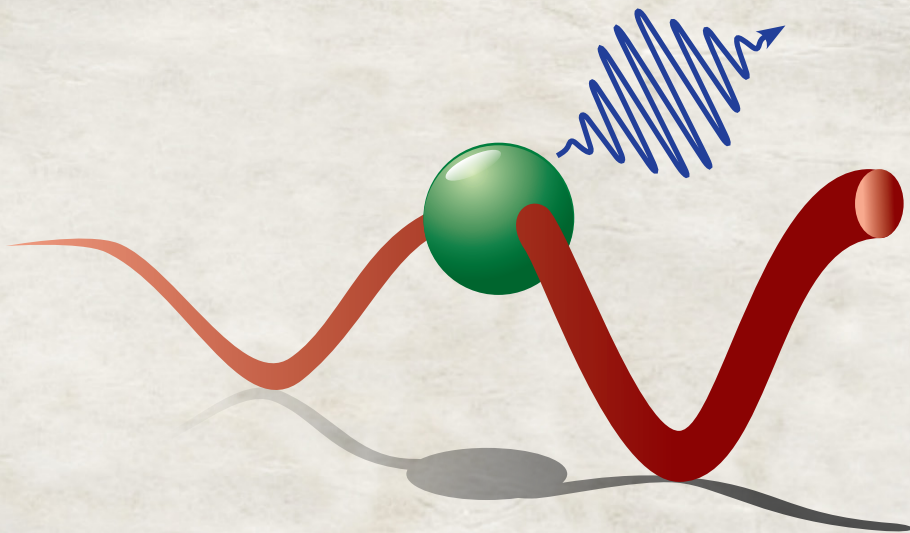

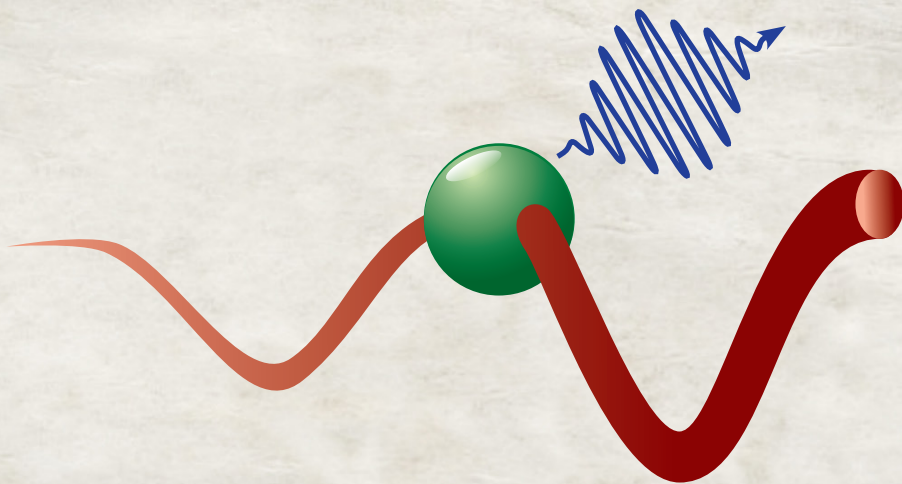

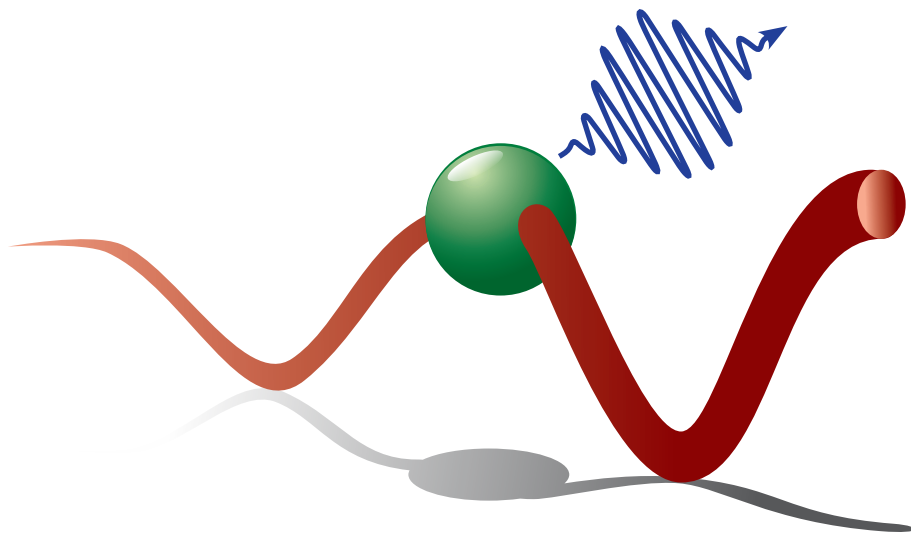

Supplement: Supplementary file 1 [file supplementary_Artwork.pdf]
